# Supplementary material for: Intrinsically Motivated Discovery of Diverse Patterns in Self-Organizing Systems
Source: arXiv:1908.06663 ancillary file (2020-02-17)
Supplement: Supplementary file 1 [file supplementary_material.pdf]

# SUPPLEMENTARY MATERIAL FOR “INTRINSICALLY MOTIVATED DISCOVERY OF DIVERSE PATTERNS IN SELF-ORGANIZING SYSTEMS”

**Chris Reinke\*, Mayalen Etcheverry\*, Pierre-Yves Oudeyer**

Flowers Team, Inria

Bordeaux, France

{chris.reinke,mayalen.etcheverry,pierre-yves.oudeyer}@inria.fr

## 1 OVERVIEW

The supplementary material lists results for additional variants of the exploration algorithms and their meta-parameter settings that were omitted in the main paper (Reinke et al., 2020). Section 2 lists results for an additional random search algorithm and variants of hand-defined goal space searches (IMGEP-HGS). Section 3 lists results for different variants of exploration algorithms based on goal spaces defined by VAEs. Several methods to define randomly initiated VAEs (IMGEP-RGS) and to define the loss function of VAEs (IMGEP-PGL and OGL) are compared. The final Section 4 provides a visualization of the analytic parameter and behavior space for the identified patterns of all major exploration algorithms.

## 2 RANDOM EXPLORATION AND IMGEPs WITH HAND-DEFINED GOAL SPACES

The main paper reports results of a standard random exploration and one IMGEP variant with a hand-defined goal space. This section provides the implementation details and diversity results of a further random exploration variant (Random Mutation) and IMGEPs with different hand-defined goal spaces.

### 2.1 RANDOM EXPLORATIONS

We evaluated two random exploration strategies: Random Initialization and Random Mutation. The main paper only discusses the Random Initialization approach.

**Random Initialization:** This approach sampled for each of the 5000 explorations a random parameter  $\theta$  including a random CPPN to generate the initial state  $A^{t=1}$ .

**Random Mutation:** This approach is closer to the principle of IMGEPs. It first performs  $N_{init} = 1000$  random explorations and adds each explored parameter  $\theta$  to a history  $\mathcal{H}$ . Afterwards, it randomly samples a parameter from the history and mutates it. The new parameter is also added to history  $\mathcal{H}$ . The approach can be replicated by using Algorithm 2 (main paper) where the parameter sampling distribution  $\mathcal{G}(\mathcal{H})$  (line 6) is selecting a random parameter from the history and mutating it.

### 2.2 IMGEPs WITH HAND-DEFINED GOAL SPACES

We evaluated several IMGEP variants with goal spaces that were hand-defined (IMGEP-HGS). Each space was constructed by a different combination (Table 1) of statistical measures of the final Lenia patterns which are described in Section B.3 of the main paper. The main paper only discusses the variant that combines all statistical measures (IMGEP-HGS 9).

---

\*Equal contribution.

| Feature            | HGS-Variants |   |   |   |   |   |   |   |   |
|--------------------|--------------|---|---|---|---|---|---|---|---|
|                    | 1            | 2 | 3 | 4 | 5 | 6 | 7 | 8 | 9 |
| mass $M_A$         | ×            | × | × | × | × | × | × | × | × |
| volume $V_A$       | ×            | × | × | × |   |   |   |   | × |
| density $D_A$      |              |   |   |   | × | × | × | × | × |
| centeredness $C_A$ |              | × |   | × |   | × |   | × | × |
| asymmetry $A_A$    |              |   | × | × |   |   | × | × | × |

Table 1: IMGEP-HGS Variants

### 2.3 RESULTS

The random explorations and IMGEP-HGS variants are compared by their resulting diversity in the analytic parameter and behavior space (Fig. 1). The diversity is measured by the number of reached bins in each space using a binning of 7 bins per dimension.

The Random Initialization approach reached for all diversity measures a higher diversity than the Random Mutation approach. Therefore, the Random Initialization approach is used for the comparison to IMGEP approaches in the main paper.

Most IMGEP-HGS variants had a higher diversity in the analytic behavior space compared to random explorations, although their diversity in the analytic parameter space is lower. This shows the advantage of IMGEPs over random searches in discovering a wider range of patterns in the target system. The best overall diversity had IMGEP-HGS 3, 4 and 9. We chose IMGEP-HGS 9 to compare it with learned goal spaces in the main paper. It identified the highest diversity of non-animals of the three variants (3, 4, 9) reaching a higher diversity for non-animals than any IMGEP with a learned goal space. It was therefore selected to show that the choice of the goal space has an influence on the patterns that IMGEPs identify.

Depending on the statistical measures used to define the goal space the diversity between the IMGEP-HGS variants varied. IMGEPs that use the volume measure (HGS 1 - 4) reach in general a higher overall diversity which can be attributed to their higher diversity of animal patterns than goal spaces with the density measure (HGS 5 - 8) (Fig. 1, b, c). In terms of diversity of identified animals showed the inclusion of several measures the best performance (HGS 4 and HGS 8 in Fig. 1, c). In terms of diversity of identified non-animals showed the inclusion of several measures besides the centeredness  $C_A$  measure the best performance (HGS 3 and HGS 7 in Fig. 1, d). The results show that the choice of the goal space has an important influence on the diversity of identified patterns and their type (animal or non-animal).

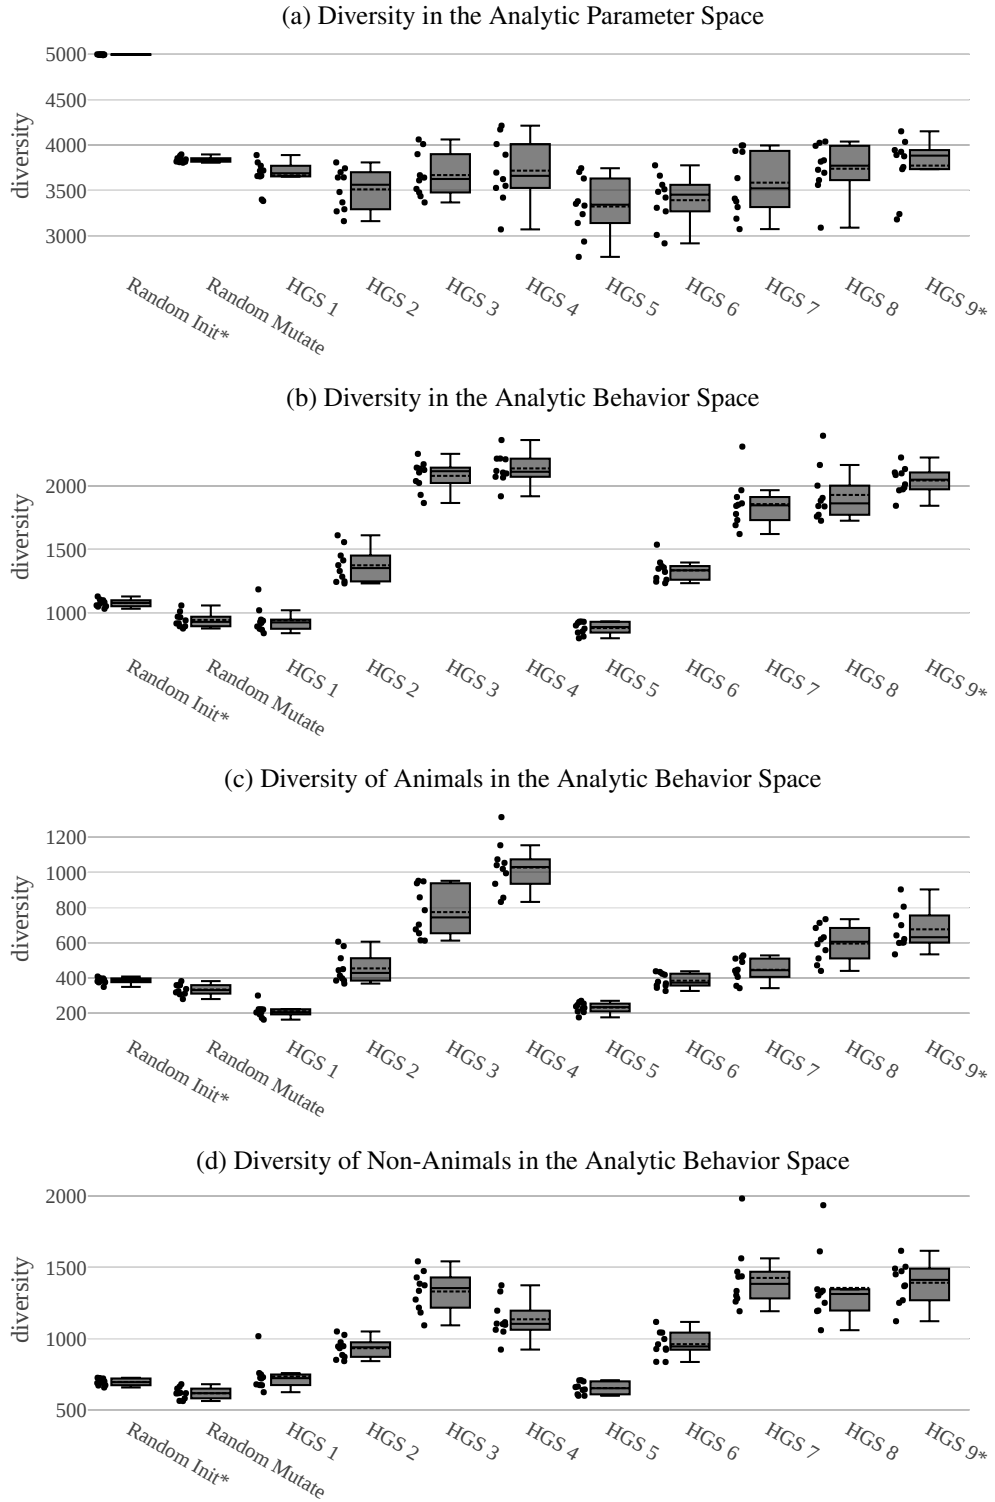

Figure 1: Although all IMGEP-HGS variants have lower diversity in the analytic parameter space compared to the Random Initialization approach, most of them have a higher diversity in the analytic behavior space. Each dot besides the boxplot shows the diversity of found patterns for each repetition ( $n = 10$ ). The box ranges from the upper to the lower quartile. The whiskers represent the upper and lower fence. The mean is indicated by the dashed line and the median by the solid line.

### 3 IMGEPs WITH RANDOM AND LEARNED GOAL SPACES USING DEEP VARIATIONAL AUTOENCODERS

We considered three random initializations for the VAE encoders used in the IMGEP-RGS. Moreover, we evaluated three different training objectives for learning the VAE goal space used in IMGEP-PGL and IMGEP-OGL. This section details the different variants and compares their diversity results.

#### 3.1 IMGEPs WITH RANDOM VAE GOAL SPACES

To study the impact of learning representations we implemented IMGEP-RGS as an ablated version of IMGEPs where the goal space is based on the encoder of a VAE with random weights. We evaluated three variants to randomly set the weights of the VAE encoder: Pytorch (Paszke et al., 2017), Xavier (Glorot & Bengio, 2010) and Kaiming (He et al., 2015). The VAE is composed of four 2D convolutional layers (with ReLU activations) followed by three fully-connected layers. Table 2 shows the different sampling distributions from which the encoder parameters are initialized. We used uniform distributions for both Xavier and Kaiming variants and set all the layers bias parameters to zero. The Xavier method was used for the results in the main paper.

| RGS Variants | bound $b$                                                           | Convolutional Layers |                      | Linear Layers        |                      |
|--------------|---------------------------------------------------------------------|----------------------|----------------------|----------------------|----------------------|
|              |                                                                     | weight               | bias                 | weight               | bias                 |
| Pytorch      | $\frac{1}{\sqrt{\text{fan}_{\text{in}}}}$                           | $\mathcal{U}(-b, b)$ | $\mathcal{U}(-b, b)$ | $\mathcal{U}(-b, b)$ | $\mathcal{U}(-b, b)$ |
| Xavier       | $\sqrt{\frac{6}{\text{fan}_{\text{in}} + \text{fan}_{\text{out}}}}$ | $\mathcal{U}(-b, b)$ | 0                    | $\mathcal{U}(-b, b)$ | 0                    |
| Kaiming      | $\sqrt{\frac{6}{\text{fan}_{\text{in}}}}$                           | $\mathcal{U}(-b, b)$ | 0                    | $\mathcal{U}(-b, b)$ | 0                    |

Table 2: IMGEP-RGS variants initialization schemes.  $\text{fan}_{\text{in}}$  is the number of input units in the weight tensor and  $\text{fan}_{\text{out}}$  is the number of output units in the weight tensor.

#### 3.2 IMGEPs WITH LEARNED VAE GOAL SPACES

The recent growing interest in unsupervised representation learning, and therefore in VAEs, resulted in a high number of proposed losses, network designs and choices of family for the encoder, decoder and prior distributions (Tschannen et al., 2018). In order to enhance desired properties such as interpretability and disentanglement of the latent variables, many current state-of-the-art approaches build on the VAE framework and augment the VAE objective (Higgins et al., 2017; Burgess et al., 2018; Kim & Mnih, 2018; Chen et al., 2018; Kumar et al., 2017). We tested the VAE architecture with three different objectives: the classical VAE objective (Kingma & Welling, 2013) (Eq. 5 of the main paper with  $\beta = 1$ ), the  $\beta$ -VAE objective (Higgins et al., 2017) (Eq. 5 of the main paper with  $\beta = 5$ ) and an augmented  $\beta$ -VAE objective (Eq. 1).

The  $\beta$ -VAE objective re-weights the  $b$  term by a factor  $\beta > 1$ , aiming to enhance the disentangling properties of the learned latent factors. We are interested in such properties as it has been shown that it can benefit exploration (Laversanne-Finot et al., 2018). However, heavily penalizing  $b$  can result in the network learning to “sacrifice” one or more of the learned latent variables in order to nullify their contribution  $b_i$  (Eq. 4 of the main paper). Those dimensions become completely uninformative and useless for further exploration in the learned latent space. This phenomenon is known as *posterior collapse* and is a common problem when training VAEs (Bowman et al., 2015; Chen et al., 2016; He et al., 2019; Kingma et al., 2016).

To prevent this phenomenon to happen, we then considered an augmented  $\beta$ -VAE objective with a new term that encourages the network to decrease *together* the individual contributions  $b_i$  of the different latent variables. This augmented loss term not only minimizes the averaged contribution (sum) but also the variance of the individual contributions:

$$b_{\text{aug}} = \sum_{i=1}^d b_i + \text{Var}([b_1, \dots, b_d]) . \quad (1)$$

Similarly other modifications of the training objective can be found in the literature to avoid posterior collapse (Tolstikhin et al., 2017; Zhao et al., 2017).

The training objective of all three evaluated VAE approaches can be given as:

$$\text{Loss}(x, \hat{x}, \mu, \sigma) = -a + \beta \left( \sum_{i=1}^d b_i + \gamma \text{Var}([b_1, \dots, b_d]) \right) \quad (2)$$

where  $x$  are the input patterns,  $\hat{x}$  are the reconstructed patterns,  $\mu, \sigma$  are the outputs of the decoder network and  $d$  is the number of latent dimensions. The hyperparameter settings of the different approaches are given in Table 3. The reconstruction accuracy part  $a$  of the loss is given by a binary cross entropy with logits. The KL divergence is defined by the terms  $b_i$ . See Section B.6.1 of the main paper for their definitions.

| VAE Variant      | $\beta$ | $\gamma$ |
|------------------|---------|----------|
| VAE              | 1       | <b>0</b> |
| $\beta$ -VAE     | 5       | <b>0</b> |
| $\beta$ -VAE aug | 5       | <b>1</b> |

Table 3: Hyperparameters for the loss function (Eq. 2) that define the three evaluated VAE variants.

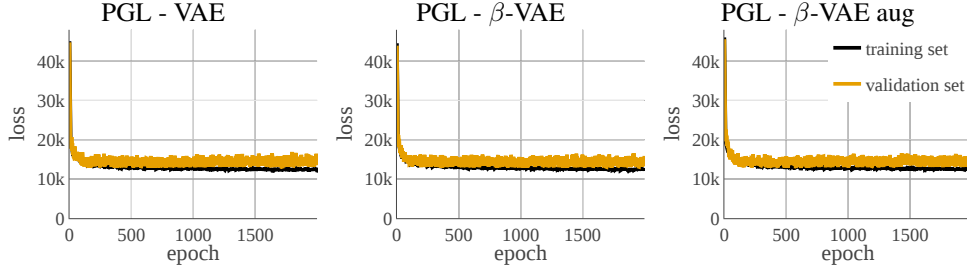

Figure 2: Averaged learning curves ( $n = 10$ ) of the VAEs for the IMGEP-PGL experiments.

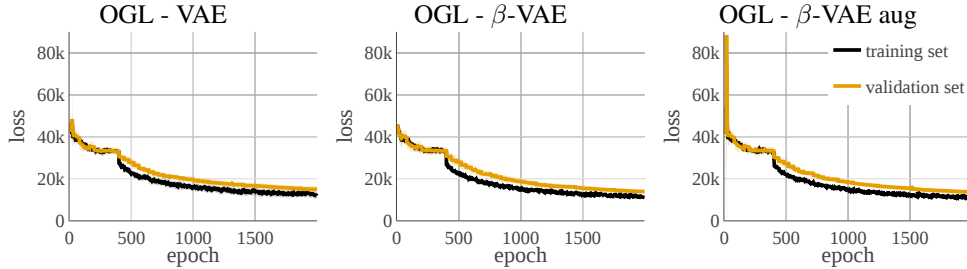

Figure 3: Averaged learning curves ( $n = 10$ ) of the VAEs for the IMGEP-OGI experiments.

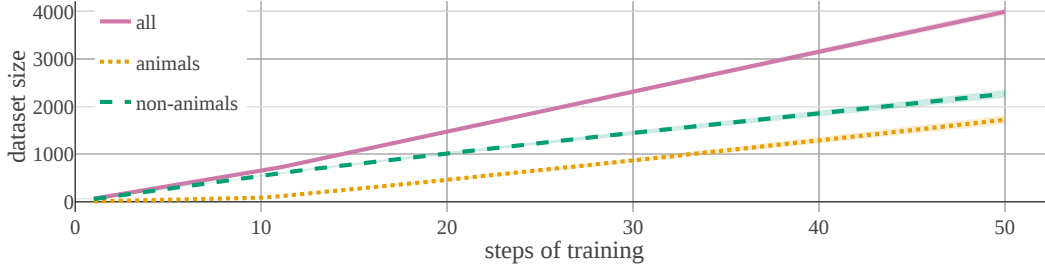

Figure 4: The IMGEPOGL collects during the exploration animal and non-animal patterns to add them to its dataset for the training of the VAE. The figure shows the development of the averaged dataset size over all repetitions ( $n = 10$ ) of the IMGEPOGL algorithm with a  $\beta$ -VAE. Standard deviation is depicted as a shaded area but it is for some not visible because it is too small.

### 3.3 RESULTS

We compared the different IMGEPRGS variants as well as the different training objective variants for IMGEPRs with learned goal spaces (PGL and OGL). The algorithms are compared by the diversity of their identified patterns in the analytic parameter and behavior space (Section B.7 of the main paper). Diversity is measured by the number of discretized bins that were explored by the algorithms in each space if each dimension of the space is separated in 7 bins.

The learning curve of the VAEs for each training objective show that all approaches are able to learn representations (Fig. 2 and 3). Fig. 4 shows the evolution of the composition of the training dataset that is collected online for the IMGEPOGL in terms of number of animals and non-animals.

All the IMGEPRs with learned goal spaces reached a higher diversity in the analytic behavior space compared to random explorations (Fig. 5, b), although random explorations have a higher diversity in the analytic parameter space (Fig. 5, a). This result confirms further the advantage of IMGEPRs over random explorations in terms of identifying diverse patterns.

Furthermore, all the IMGEPRs with learned goal spaces outperformed the IMGEPR with random goal space. This result shows the importance of learning relevant pattern features that, combined with an effective exploration process, is key to discover a high diversity of patterns.

There is no significant differences between Xavier and Kaiming IMGEPRGS variants. They both seem to present a higher variance than the Pytorch variant and reach therefore a higher average performance, but it is unclear why. Because the Xavier initialization performed slightly the best for IMGEPRGS, it was used for the results in the main paper.

The difference between the PGL and OGL variants were small for all diversity measures. The OGL showed a slight advantage over the PGL versions in all diversity measures. Thus, an online version of the IMGEPR can learn an appropriate goal space during the exploration. A precollected dataset as for the PGL is not necessary to successfully use IMGEPRs.

The difference between the VAE objective variants (VAE,  $\beta$ -VAE and augmented  $\beta$ -VAE) was very small. The  $\beta$ -VAE was slightly better than the other two variants for the diversity in the analytic parameter space and for both IMGEPR variants. All VAEs seemed to learn similar features for our datasets. It might be possible that the different VAE variants show different behaviors if their parameters are fine-tuned, such as the  $\beta$  parameter, but this was out of the scope of this paper. Because the  $\beta$ -VAE objective performed slightly better for IMGEPR-PGL and IMGEPOGL, it was used for the results in the main paper.

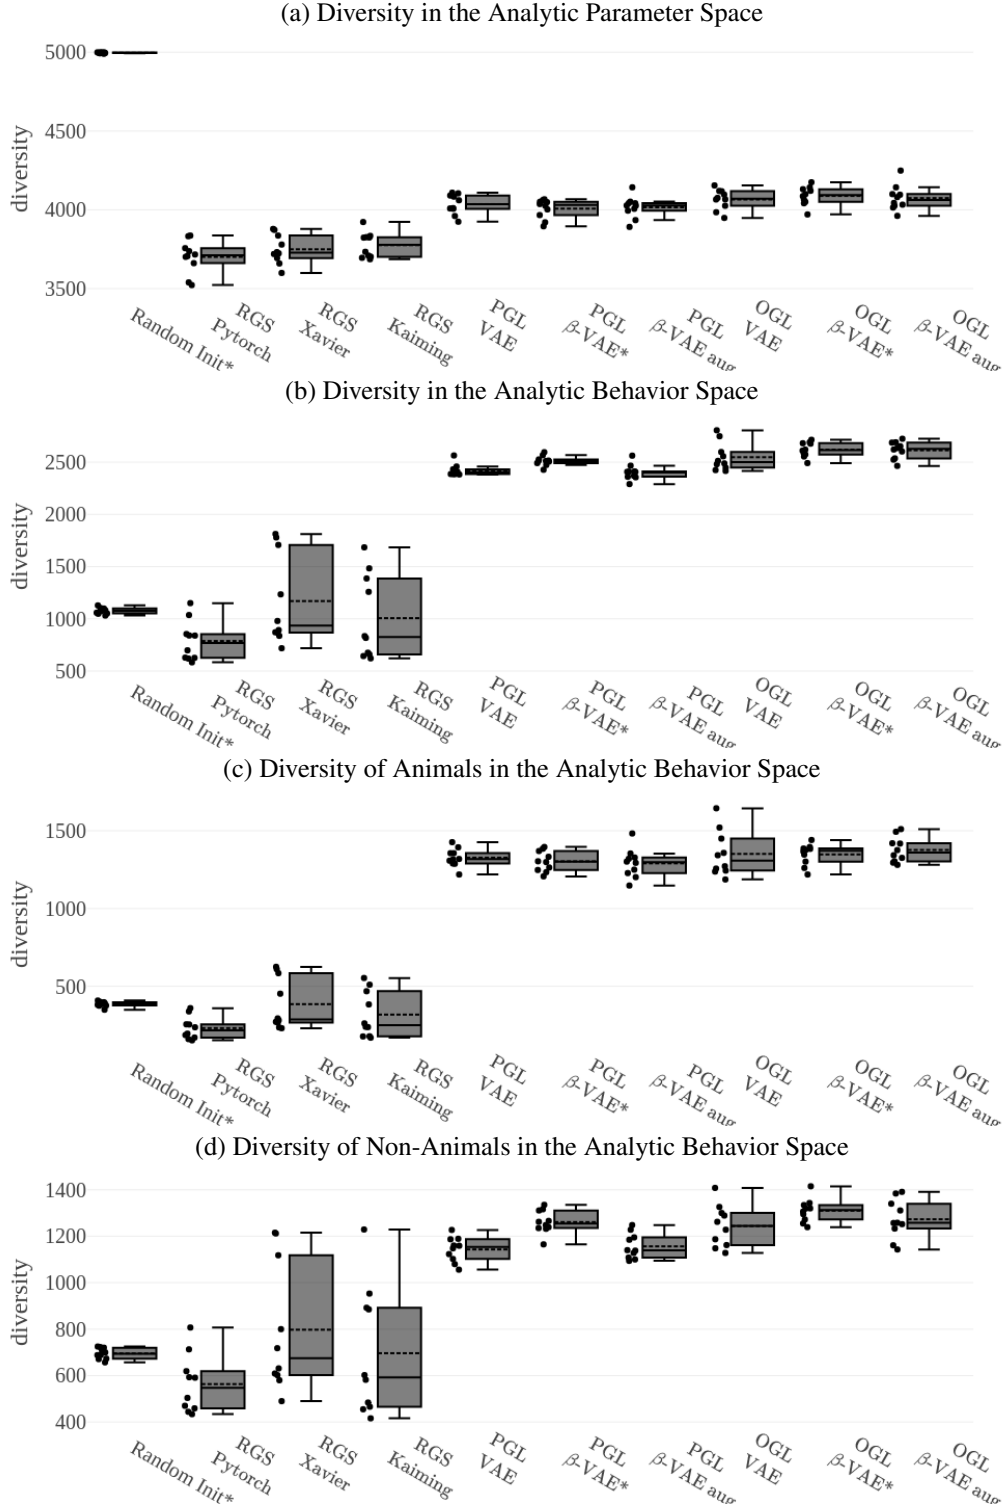

Figure 5: Trained VAE representations outperform random representations in terms of diversity, showing the importance of learning the correct features of a goal space. Each dot besides the boxplot shows the diversity of found patterns for each repetition ( $n = 10$ ). The box ranges from the upper to the lower quartile. The whiskers represent the upper and lower fence. The mean is indicated by the dashed line and the median by the solid line.

#### 4 ADDITIONAL RESULTS: DIMENSION REDUCTION OF THE ANALYTIC PARAMETER AND BEHAVIOR SPACE

A two-dimensional reduction of the identified patterns in the analytic parameter and behavior space (Section B.7 in the main paper) visualizes the diversity of the parameters and identified patterns. The results for the five exploration algorithm variants which are discussed in the main paper are given.

The dimension reduction of the parameter space is based on all explored parameters encoded in the analytic parameter space from the first repetition experiment for each algorithm. All encoded points were normalized so that the overall minimum value became 0 and the maximum value 1 for each dimension. Afterwards a principle component analysis (PCA) was performed to detect the 2 principle components (Jolliffe, 1986). The found patterns for each algorithm are plotted according to those components.

The results show that the random exploration has a stronger uniform distribution than any of the IMGEP algorithms in the analytic parameter space (Fig. 6). The IMGEP algorithms show concentrations of explorations in specific regions of the parameter space. The visualization shows also that it is not possible to define distinct regions in the parameter space that allow to differentiate between dead, animal and non-animal patterns.

The same analysis was performed for the identified patterns of each algorithm encoded in the analytic behavior space (Fig. 7). It is visible that the random exploration and the random goal space (RGS) approaches are more concentrated compared to the hand-defined (HGS) or learned goal spaces approaches (PGL and OGL), especially in a region with many non-animal patterns (north-west). The IMGEP-RGS has a similar spread than random exploration, with an even higher concentration of non-animals (north-west). The IMGEP-HGS has a wider spread in the non-animal area. The IMGEPs with a learned goal space (PGL and OGL) show a stronger distribution in an area that encodes mostly animals (south).

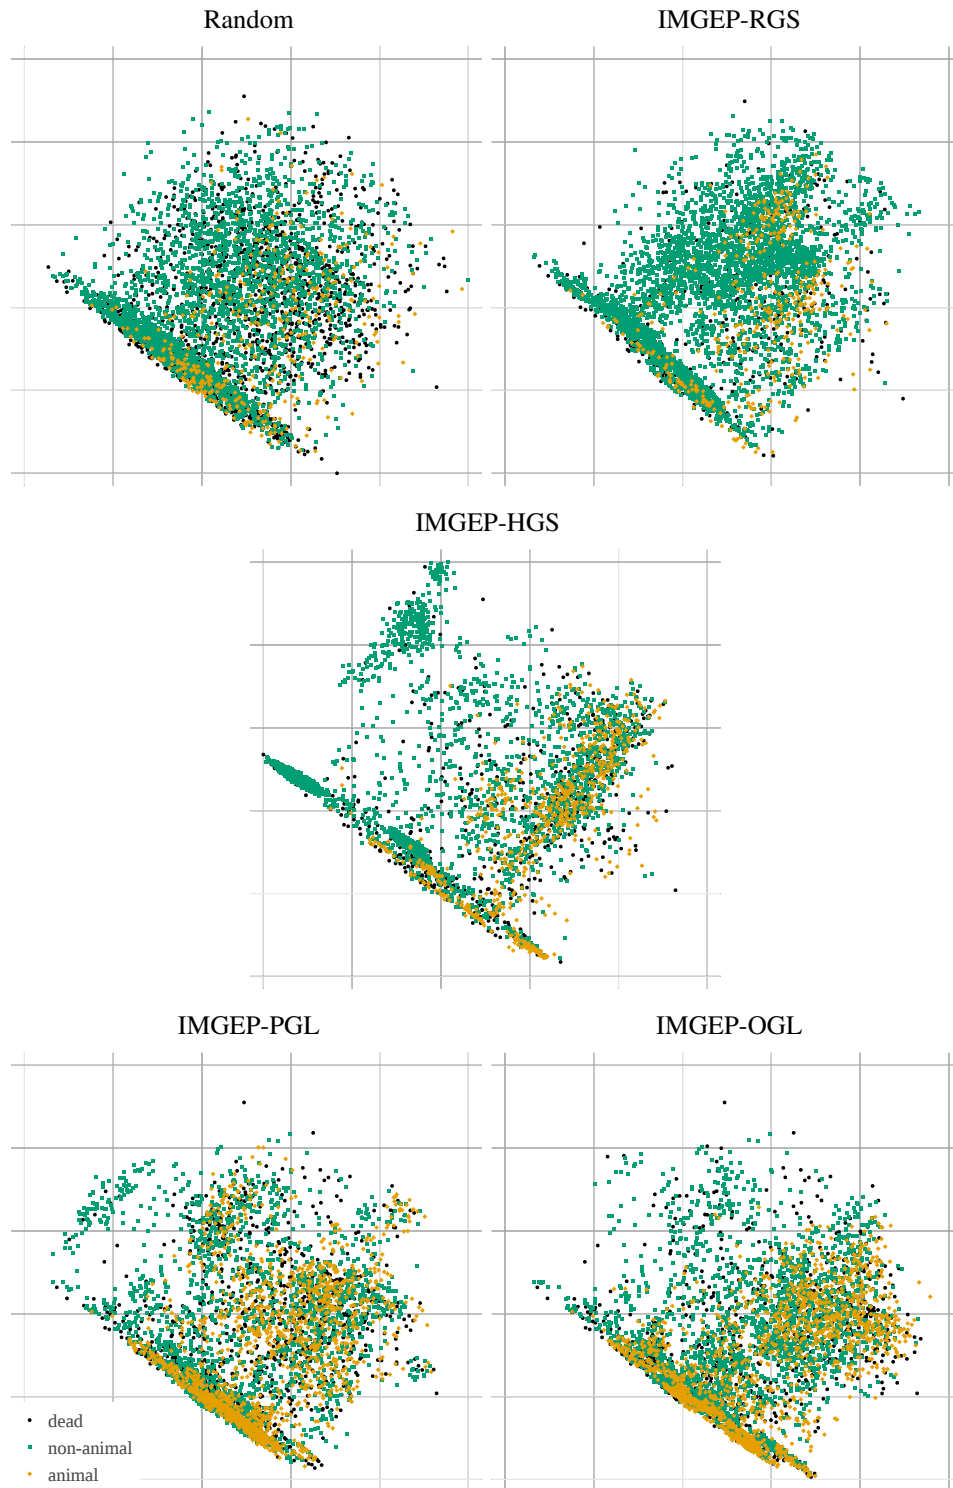

Figure 6: A random exploration covers the analytic parameter space more uniformly than IMGEP algorithms which form clusters at certain areas. PCA dimension reduction of the analytic parameter space which illustrates all explored parameters by the first repetition experiment per algorithm.

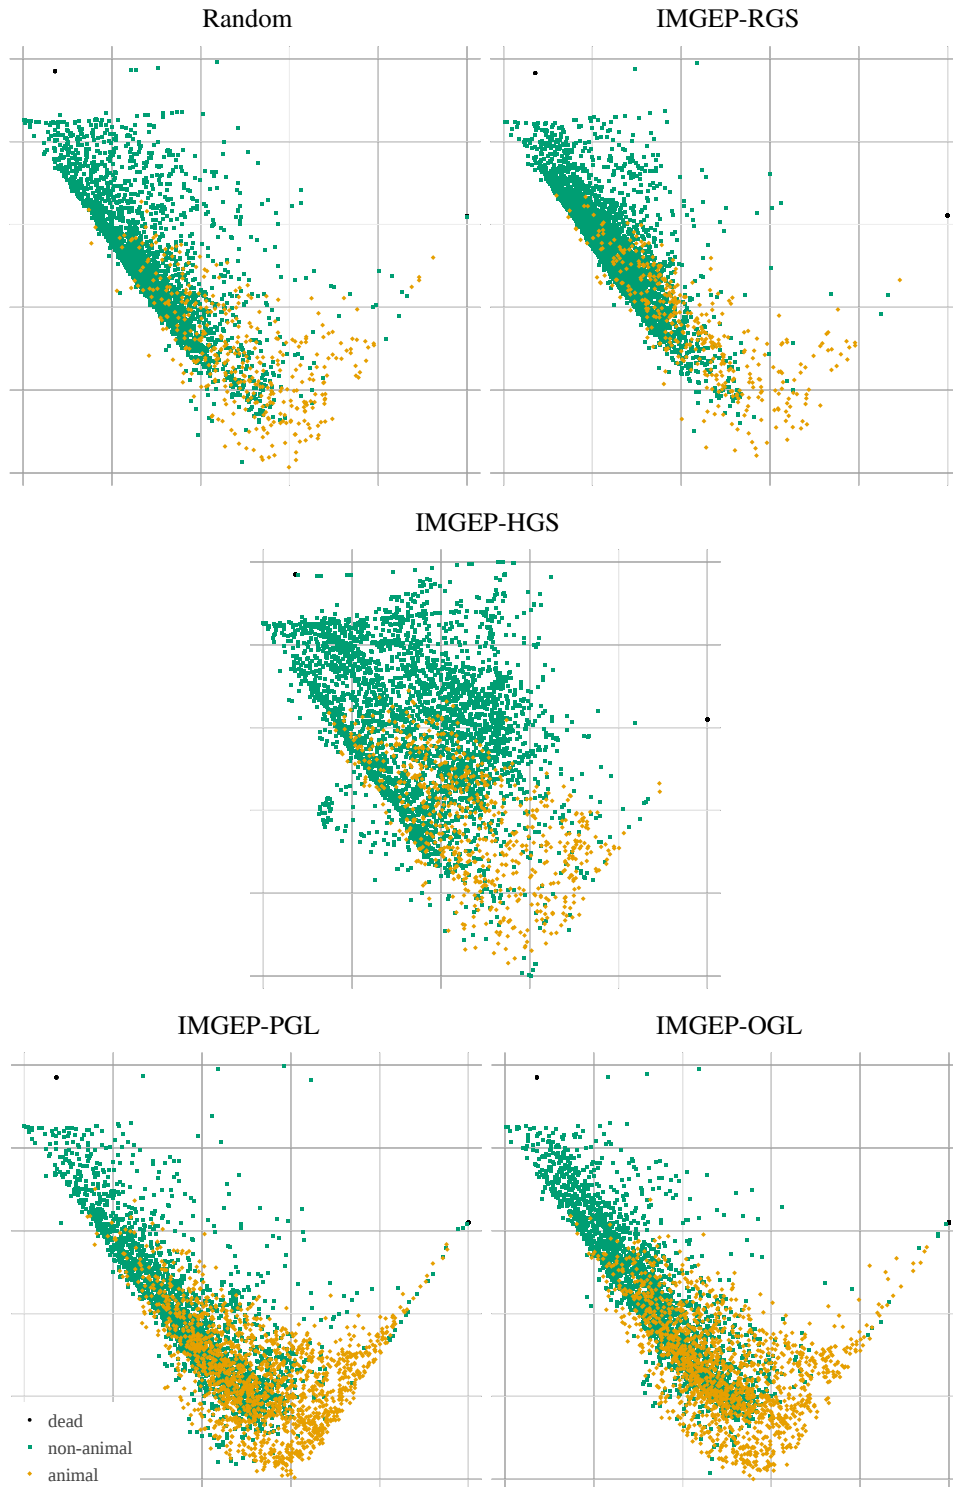

Figure 7: In the analytic behavior space IMGEPs reach a higher diversity compared to a random exploration, except IMGEP-RGS which covers similar areas. The HGS approach explores more non-animal areas and the PGL and OGL more animal areas. PCA dimension reduction of the analytic behavior space which illustrates all identified patterns by the first repetition experiment per algorithm.

## REFERENCES

- Samuel R Bowman, Luke Vilnis, Oriol Vinyals, Andrew M Dai, Rafal Jozefowicz, and Samy Bengio. Generating sentences from a continuous space. *arXiv preprint arXiv:1511.06349*, 2015.
- Christopher P Burgess, Irina Higgins, Arka Pal, Loic Matthey, Nick Watters, Guillaume Desjardins, and Alexander Lerchner. Understanding disentangling in *beta*-vae. *arXiv preprint arXiv:1804.03599*, 2018.
- Tian Qi Chen, Xuechen Li, Roger B Grosse, and David K Duvenaud. Isolating sources of disentanglement in variational autoencoders. In *Advances in Neural Information Processing Systems*, pp. 2610–2620, 2018.
- Xi Chen, Diederik P Kingma, Tim Salimans, Yan Duan, Prafulla Dhariwal, John Schulman, Ilya Sutskever, and Pieter Abbeel. Variational lossy autoencoder. *arXiv preprint arXiv:1611.02731*, 2016.
- Xavier Glorot and Yoshua Bengio. Understanding the difficulty of training deep feedforward neural networks. In *Proceedings of the thirteenth international conference on artificial intelligence and statistics*, pp. 249–256, 2010.
- Junxian He, Daniel Spokoyny, Graham Neubig, and Taylor Berg-Kirkpatrick. Lagging inference networks and posterior collapse in variational autoencoders. *arXiv preprint arXiv:1901.05534*, 2019.
- Kaiming He, Xiangyu Zhang, Shaoqing Ren, and Jian Sun. Delving deep into rectifiers: Surpassing human-level performance on imagenet classification. In *Proceedings of the IEEE international conference on computer vision*, pp. 1026–1034, 2015.
- Irina Higgins, Loic Matthey, Arka Pal, Christopher Burgess, Xavier Glorot, Matthew Botvinick, Shakir Mohamed, and Alexander Lerchner. *beta*-vae: Learning basic visual concepts with a constrained variational framework. In *International Conference on Learning Representations*, volume 3, 2017.
- I. T. Jolliffe. *Principal Component Analysis and Factor Analysis*, pp. 115–128. Springer New York, New York, NY, 1986. ISBN 978-1-4757-1904-8. doi: 10.1007/978-1-4757-1904-8\_7.
- Hyunjik Kim and Andriy Mnih. Disentangling by factorising. *arXiv preprint arXiv:1802.05983*, 2018.
- Diederik P Kingma and Max Welling. Auto-encoding variational bayes. *arXiv preprint arXiv:1312.6114*, 2013.
- Durk P Kingma, Tim Salimans, Rafal Jozefowicz, Xi Chen, Ilya Sutskever, and Max Welling. Improved variational inference with inverse autoregressive flow. In *Advances in neural information processing systems*, pp. 4743–4751, 2016.
- Abhishek Kumar, Prasanna Sattigeri, and Avinash Balakrishnan. Variational inference of disentangled latent concepts from unlabeled observations. *arXiv preprint arXiv:1711.00848*, 2017.
- Adrien Laversanne-Finot, Alexandre Pere, and Pierre-Yves Oudeyer. Curiosity driven exploration of learned disentangled goal spaces. In Aude Billard, Anca Dragan, Jan Peters, and Jun Morimoto (eds.), *Proceedings of The 2nd Conference on Robot Learning*, volume 87 of *Proceedings of Machine Learning Research*, pp. 487–504. PMLR, 29–31 Oct 2018.
- Adam Paszke, Sam Gross, Soumith Chintala, Gregory Chanan, Edward Yang, Zachary DeVito, Zeming Lin, Alban Desmaison, Luca Antiga, and Adam Lerer. Automatic differentiation in pytorch. In *NIPS-W*, 2017.
- Chris Reinke, Mayalen Etcheverry, and Pierre-Yves Oudeyer. Intrinsically motivated discovery of diverse patterns in self-organizing systems. In *International Conference on Learning Representations*, 2020.

Ilya Tolstikhin, Olivier Bousquet, Sylvain Gelly, and Bernhard Schoelkopf. Wasserstein auto-encoders. *arXiv preprint arXiv:1711.01558*, 2017.

Michael Tschannen, Olivier Bachem, and Mario Lucic. Recent advances in autoencoder-based representation learning. *arXiv preprint arXiv:1812.05069*, 2018.

Shengjia Zhao, Jiaming Song, and Stefano Ermon. Infovae: Information maximizing variational autoencoders. *arXiv preprint arXiv:1706.02262*, 2017.
